# Supplementary material for: Hybrid approach predicts a lower binding energy for benzene on water ice
Source: arXiv:2406.19117 source file (2024-06-27)
Supplement: Supplementary file 1 [file Clark-Benoit-VandeSande-Walsh-SI.pdf]

# Supplementary information for Hybrid approach predicts a lower binding energy for benzene on water ice

Victoria H.J. Clark,[1★] David M. Benoit,[2†] Marie Van de Sande,[3,4‡] and Catherine Walsh[3§]
[1] *Department of Physics and Astronomy, University College London, London, WC1E 6BT, UK*
[2] *E.A. Milne Centre for Astrophysics, University of Hull, Hull, HU6 7RX, UK*
[3] *School of Physics and Astronomy, University of Leeds, Leeds, LS2 9JT, UK*
[4] *Leiden Observatory, Leiden University, P.O. Box 9513, 2300 RA Leiden, The Netherlands*

26 June 2024

## BASIS-SET SUPERPOSITION ERROR (BSSE) ESTIMATION FOR THE BINDING ENERGY

In order to estimate the influence of BSSE on the binding energy of the benzene–water cluster, the water dimer and benzene adsorbed on water ice XIh, we performed a counterpoise correction estimation following van Duijneveldt et al. (1994). Here, as in the main paper, we define the binding energy of a benzene molecule as a negative quantity, but this time including a BSSE energy correction:

$$D_{e\,(\mathrm{Bz-Ice})} = E_{(\mathrm{Bz-Ice,opt})} - \left[E_{(\mathrm{Ice,opt})} + E_{(\mathrm{Bz,opt})}\right] + E^{\mathrm{high}}_{\mathrm{model,BSSE}}(\mathrm{Ice, Bz}) \tag{1}$$

where the opt label refers to an optimisation at the PBE-D3/MOLOPT-TZV2P level of theory, $E_{(\mathrm{Bz-Ice,opt})}$ refers to the bound benzene on ice, $E_{(\mathrm{Ice,opt})}$ refers to the pure ice surface and $E_{(\mathrm{Bz,opt})}$ refer to the gaseous benzene structure. Each component on the right of Equation (1) above is then computed using a two-level ONIOM approach such that

$$E_{(\mathrm{Bz-Ice,opt})} = E^{\mathrm{low}}_{(\mathrm{Bz-Ice,opt})} - \left[E^{\mathrm{low}}_{(\mathrm{model})} + E^{\mathrm{high}}_{(\mathrm{model})}\right], \tag{2}$$

$$E_{(\mathrm{Ice,opt})} = E^{\mathrm{low}}_{(\mathrm{Ice,opt})} - \left[E^{\mathrm{low}}_{(\mathrm{ice\ model})} + E^{\mathrm{high}}_{(\mathrm{ice\ model})}\right], \tag{3}$$

$$E_{(\mathrm{Bz,opt})} = E^{\mathrm{high}}_{(\mathrm{Bz,opt})}. \tag{4}$$

The purpose of the BSSE term in eq. 1 is to correct the high-level results for basis-set incompleteness. We only correct this for the high-level model since this is the site of the interaction. We reformulate the traditional BSSE correction and monomer deformation equations into our overall BSSE correction term below, so that we can conserve the formal expression of eq. 1. If we label the basis set used for the ice model as $A$, the basis set used to describe benzene by $B$ and the joint basis set as $A \cup B$, the BSSE-correction term can be defined as

$$E^{\mathrm{high}}_{\mathrm{model,BSSE}}(\mathrm{Ice, Bz}) = \left[E^{\mathrm{high}}_{(\mathrm{ice\ model})}(A) - E^{\mathrm{high}}_{(\mathrm{ice\ model})}(A \cup B)\right] + \left[E^{\mathrm{high}}_{(\mathrm{Bz})}(B) - E^{\mathrm{high}}_{(\mathrm{Bz})}(A \cup B)\right], \tag{5}$$

where, the geometries of each fragment (ice and benzene) is kept at the optimised geometry for bound benzene on ice, by definition. Here, as in the main manuscript, the high-level calculations are defined as DLPNO-CCSD(T)/EC2-ANO-CBS(2,3) calculation.

The results are obtained using the same composite approach as the one outlined in the main paper (see also eq. 1 and are shown in Table 1). We see that for all complexes studied: benzene–water, water dimer and benzene–ice (XIh), the difference in predicted binding energy remains small ($\ll$ 1 kJ/mol).

We also computed the deformation energy occurring during the formation of the binding complex. Those values are defined as $E$(complex geometry)−

**Table 1.** Computed binding energies for benzene-$H_2O$, the water dimer and benzene–ice(XIh). Values are given in kJ/mol. BSSE-corrected values are indicated by the label "[BSSE]". Both benzene-water and water dimer use the cluster geometries from the S22 database (obtained from www.begdb.com (Řezáč et al. 2008)).

| System | Method | Binding energy [kJ/mol] |
|---|---|---|
| Benzene–$H_2O$ cluster | | |
| | DLPNO-CCSD(T)/EC2-CBS(2,3) | −13.52 |
| | DLPNO-CCSD(T)/EC2-CBS(2,3) [BSSE] | −13.47 |
| $H_2O$–$H_2O$ cluster | | |
| | DLPNO-CCSD(T)/EC2-CBS(2,3) | −20.35 |
| | DLPNO-CCSD(T)/EC2-CBS(2,3) [BSSE] | −19.98 |
| Benzene–ice (XIh) | | |
| | DLPNO-CCSD(T)-hybrid/CBS(2,3) | −35.62 |
| | DLPNO-CCSD(T)-hybrid/CBS(2,3) [BSSE] | −36.20 |

© 0000 The Authors

$E$(optimised geometry), with a positive value expected to indicate that there is a large rearrangement of the molecular structure upon binding (adsorption). The values obtained for the fragments of the benzene on ice complex are: +9.22 kJ/mol for the ice XIh layer model and +11.36 kJ/mol for the benzene molecule. Note that, as in the main manuscript, we use the DLPNO-CCSD(T)/EC2-ANO-CBS(2,3) level of theory and those values are obtained for the model parts of the system only.

## REFERENCES

Řezáč J., et al., 2008, Collect. Czechoslov. Chem. Commun., 73, 1261
van Duijneveldt F. B., van Duijneveldt-van de Rijdt J. G. C. M., van Lenthe J. H., 1994, Chemical Reviews, 94, 1873–1885
